# Supplementary material for: Solvent reaction coordinate for an S$_N$2 reaction
Source: arXiv:2007.04126 ancillary file (2020-07-08)
Supplement: Supplementary file 1 [file supplementary_material.pdf]

# Supplementary Material: Solvent reaction coordinate for an $S_N2$ reaction

Christian Leitold,[1,2] Christopher J. Mundy,[3] Marcel D. Baer,[3] Gregory K. Schenter,[3] and Baron Peters[1,4]
[1)]*Department of Chemical and Biomolecular Engineering, University of Illinois at Urbana-Champaign, 61801, USA*
[2)]*Faculty of Physics, University of Vienna, 1090 Wien, Austria (present affiliation)*
[3)]*Physical Sciences Division, Pacific Northwest National Laboratory, Richland, WA 99352, USA*
[4)]*Department of Chemistry and Biochemistry, University of Illinois at Urbana-Champaign, 61801, USA*

(Dated: April 8, 2020)

## I. GAS-PHASE ELECTRONIC STRUCTURE CALCULATIONS

We have performed gas-phase calculations using Gaussian 16[1] to study the effect of the chosen DFT exchange-correlation functional on the computed barrier height (Fig. 1). A TZVP basis set was employed in all calculations. For the three DFT calculations (utilizing the BLYP, B3LYP, and $\omega$B97X-D functional), we have performed a constrained geometry optimization at each prescribed value of Jorgensen's coordinate $r_J$. For CCSD(T), we have done single-point calculations at the respective optimized geometries obtained from the $\omega$B97X-D calculation. The barrier height increases significantly with increasing theory level. We hypothesize that the same trend holds true for the full system in solution, explaining the roughly 10 kcal/mol difference in barrier height between our study and previous values from the literature.

## II. HYDROGEN CHARGES ALONG $r_J$

In analogy to Fig. 2 of the main text, in Fig. 2 we show the average per-atom charge on the three hydrogen atoms in the methyl chloride molecule, given a fixed value of Jorgensen's coordinate $r_J$. Note how the charges barely deviate from an average value of $q/\mathrm{e} \approx 0.16$. On the scale of Fig. 2 of the main text, one would only see a flat line.

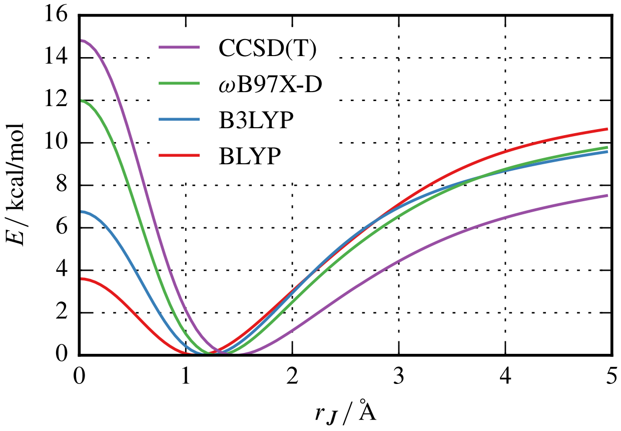


Figure 1. Barrier height of the gas-phase reaction for different theory levels. All curves have been shifted so that the energy minimum is $E_{\min} = 0$.

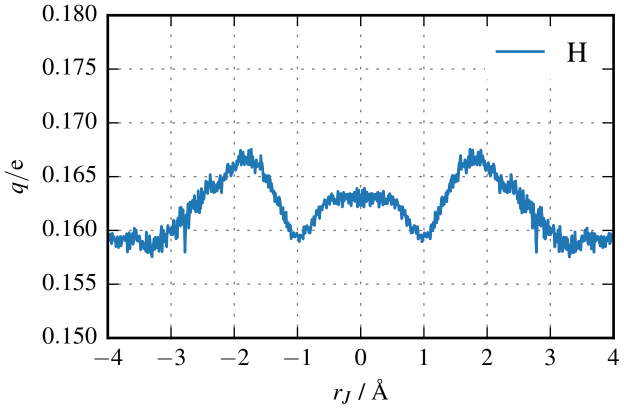


Figure 2. Average Mulliken charge on the hydrogen atoms along $r_J$.

## III. EPF PROCEDURE

In Fig. 3, we show randomly selected trajectories from the EPF calculation to obtain the transmission coefficient $\kappa$. This procedure minimizes the amount of CPU time spent on trajectories that contribute zero to the average, as for the most part, these trajectories can be terminated early. In the case of a violation of the *positive* condition, which on average will occur for half of the sampled configurations, there is not even a need to start a trajectory at all.

## IV. LOG LIKELIHOOD RESULTS

In Table I, we show all inertial log likelihood scores, including these for additional variable combinations not discussed in the main text. We have also included a trial coordinate based on the "pinching coordinate" $\Delta c_H$. In the case of $\Delta c_H$, an additional optimization has to be performed, in order to determine the two parameters of the cutoff function used in the definition of the coordination numbers, Eq. (17) in the main text. Given the results observed for the other trial coordinates, we have performed this type of full optimization only for the

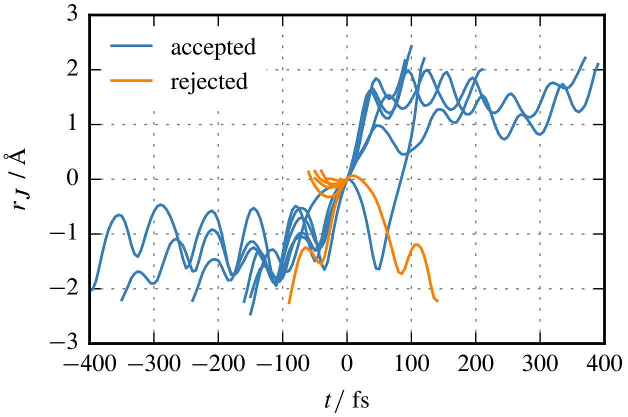


Figure 3. Sample trajectories from the EPF calculation. Most rejections happen early, because either the *positive* or the *first* condition is violated.

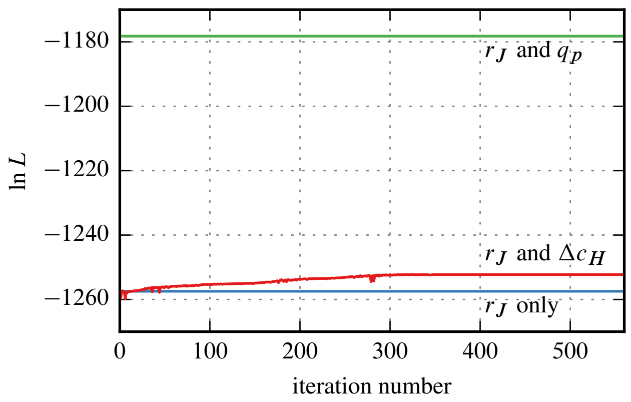


Figure 4. (Red line) Likelihood optimization for the “pinching coordinate” $\Delta c_H$ in combination with $r_J$. As a reference point, we show the likelihood scores for $r_J$ as the only coordinate, as well as for its combination with the $q_p$ solvent coordinate. Due to the need to re-calculate all coordination numbers for many thousands of system configurations at each iteration, this takes a little under an hour to run on a single core of a typical PC.

combination of Jorgensen's coordinate $r_J$ and the pinching coordinate $\Delta c_H$. Due to the need to re-calculate coordination numbers at each iteration, this variant of the likelihood maximization procedure is considerably slower than merely optimizing the linear coefficients $\alpha_i$ and prefactors $a$ and $b$, as done before. However, for our rather small data set, the full optimization still takes under an hour on a single CPU core of a standard workstation. The optimized result (for the same data set as presented in Table I) is a log likelihood score of -1252.3. As seen in Fig. 4, the improvement we get by including coordination numbers to quantify the solvent effects is not nearly as good as the one from the addition of our new charge-based solvent coordinate $q_p$ and some of its variants.

| | $\ln L$ | $\Delta \ln L/\Delta_{\min}$ | $\kappa$ |
|---|---|---|---|
| $r_p$, $r_J$, and $q_p$ | -1159.5 | 23.56 | - |
| $r_J$ and $q_p$ | -1178.2 | 19.04 | 0.32 ± 0.07 |
| $r_J$ and $q_{ps}$ | -1183.7 | 17.74 | - |
| $r_J$ and $q'_{ps}$ | -1192.0 | 15.74 | - |
| $r_p$ and $q_p$ | -1200.2 | 13.77 | - |
| $r_p$ and $q'_p$ | -1210.2 | 11.35 | - |
| $r_p$ and $q_{ps}$ | -1213.5 | 10.58 | - |
| $r_p$ and $q'_{ps}$ | -1216.6 | 9.82 | - |
| $r_p$ and $r_J$ | -1237.0 | 4.92 | 0.33 ± 0.08 |
| $r_J$ and $\Delta c_H$ * | -1252.3 | 1.36 | - |
| $r_J$ only | -1257.5 | 0.00 | 0.39 ± 0.07 |
| $r_J$ and $q'_p$ | -1257.0 | 0.11 | - |
| $r_p$ only | -1269.2 | -2.82 | 0.32 ± 0.05 |
| $q_p$ only | -2743.2 | -357.17 | 0 |

Table I. Optimized inertial log likelihood scores for the different candidate reaction coordinates, and the corresponding transmission coefficient $\kappa$ of the coordinates for which we have calculated it. $\Delta \ln L$ is calculated with respect to using Jorgensen's coordinate $r_J$ only.
*Additional optimization performed for this combination, see text and Fig. 4.

## REFERENCES

[1]M. J. Frisch *et al.*, Gaussian 16, Gaussian Inc. Wallingford CT, 2016.
